# Supplementary material for: Seen but Not Connected: Recovering Vessel Trees Below the Threshold
Source: arXiv:2611.38115 source file (2026-11-27)
Supplement: Supplementary file 1 [file 0_map.tex]

\providecolor{ridger}{RGB}{252,234,230}\providecolor{subhead}{gray}{0.96}
\makeatletter\@ifundefined{details}{\newenvironment{details}{\par\smallskip\begingroup\footnotesize\def\paragraph##1{\par\smallskip\noindent\textbf{##1} \ignorespaces}\noindent\textbf{Details.}\par\nobreak\noindent\ignorespaces}{\par\endgroup\smallskip}}{}\makeatother
\section*{Overview}
\label{S-sec:supp-0_map}

This appendix gives the method details, the proofs, the protocols and the full results behind the main text. It follows the order of the main text, and each section names the part of the main text that it supports. Paragraphs marked \emph{Details}, in smaller type, hold protocols and secondary analyses. Tables and figures here are numbered S1, S2, and so on; main-text tables keep their numbers.

{\makeatletter\setcounter{tocdepth}{1}\small
\renewcommand*\l@section{\@dottedtocline{1}{0em}{2.3em}}
\renewcommand*\l@subsection{\@dottedtocline{2}{0.9em}{3.0em}}
\def\numberline#1{#1\hskip 1em}%
\tableofcontents\makeatother}
\setcounter{tocdepth}{2}%
